# Supplementary material for: On Inter-dataset Code Duplication and Data Leakage in Large Language Models
Source: arXiv:2401.07930 source file (2024-08-01)
Supplement: Supplementary file 1 [file appendices.tex]

\clearpage
\appendices
\section{Layer-wise performances}

\begin{table*}[t]
\caption{Average layer-wise performances of \unixcoder{} and \graphcodebert{} for the task of code search.}
\label{tab:performancecodesearchlayer}
    \centering
\scalebox{0.8}{
\begin{tabular}{lccccc}
\toprule
        Model &  Layer &   Biased group &  Unbiased group &  Performance &  Difference \\
\hline
\graphcodebert{} &      3 & 89.16 &   88.79 & 88.84 &  0.37 \\
\graphcodebert{} &      4 & 89.28 &   88.77 & 88.83 &  0.51 \\
\graphcodebert{} &      2 & 89.26 &   88.76 & 88.83 &  0.50 \\
\graphcodebert{} &      1 & 89.31 &   88.69 & 88.77 &  0.62 \\
\graphcodebert{} &      5 & 89.40 &   88.64 & 88.74 &  0.76 \\
\graphcodebert{} &      6 & 89.40 &   88.50 & 88.61 &  0.90 \\
\graphcodebert{} &      7 & 89.10 &   88.41 & 88.50 &  0.69 \\
\graphcodebert{} &      8 & 89.03 &   88.28 & 88.37 &  0.75 \\
\graphcodebert{} &      9 & 88.89 &   88.11 & 88.21 &  0.78 \\
\graphcodebert{} &     10 & 88.78 &   87.94 & 88.05 &  0.84 \\
\graphcodebert{} &     11 & 88.11 &   86.92 & 87.07 &  1.20 \\
    \unixcoder{} &      1 & 82.47 &   81.00 & 81.19 &  1.47 \\
    \unixcoder{} &      2 & 82.44 &   80.79 & 81.00 &  1.65 \\
    \unixcoder{} &      3 & 82.44 &   80.66 & 80.89 &  1.78 \\
    \unixcoder{} &      4 & 82.58 &   80.63 & 80.88 &  1.95 \\
    \unixcoder{} &      5 & 82.59 &   80.60 & 80.86 &  1.99 \\
    \unixcoder{} &      6 & 82.45 &   80.58 & 80.82 &  1.87 \\
    \unixcoder{} &      7 & 82.63 &   80.43 & 80.72 &  2.20 \\
    \unixcoder{} &      8 & 82.39 &   79.98 & 80.29 &  2.41 \\
    \unixcoder{} &      9 & 81.77 &   79.50 & 79.79 &  2.27 \\
    \unixcoder{} &     10 & 81.09 &   78.76 & 79.06 &  2.32 \\
    \unixcoder{} &     11 & 79.06 &   76.71 & 77.01 &  2.35 \\
\bottomrule
\end{tabular}
}
\end{table*}
